# Supplementary material for: Role of vector self-interaction in Neutron Star properties
Source: arXiv:2209.12657 ancillary file (2023-12-12)
Supplement: Supplementary file 1 [file description_to_data_files.pdf]

# Description to ancillary files: “Role of vector self-interaction in Neutron Star properties”

We have included the data files as ‘ancillary files’ for all the figures in the manuscript. A comprehensive description of each data file is provided below:

- **Figure 1:**

**For Figure 1a, 1b, and 1c:** The mean meson field strengths for  $\sigma$ ,  $\omega$ , and  $\rho$  meson in the neutron star (NS) matter with different  $\zeta$  values are given in sub-folder “Fig1a1band1c”. Files are named corresponding to the values of  $\zeta$ , e.g., Meson field strengths with  $\zeta = 0.01$  can be plotted using the data from the file named ‘Meson\_fields\_PCSB1\_zeta\_0.01.out.’.

The columns of the data files can be accessed as,

$$\#1. n_b/n_0, \#2. n_b \text{ (fm}^{-3}\text{)}, \#3. \sigma \text{ (MeV)}, \#4. \omega \text{ (MeV)}, \#5. \rho \text{ (MeV)}$$

$n_b$  is the baryon density, and  $n_0$  is the saturation density.

**For Figure 1d:** The particle fraction ( $Y_i$ ) for the constituent ‘i’ in the neutron star matter with different  $\zeta$  values are given in sub-folder “Fig1d”. Files are named corresponding to the values of  $\zeta$ , e.g., particle fraction with  $\zeta = 0.01$  can be plotted using the file ‘Particle\_fraction\_zeta\_0.01.out’.

Where,

$$(i = \{\text{proton}(p), \text{neutron}(n), \text{electron}(e^-), \text{muon}(\mu^-)\})$$

The columns of the data files can be read as,

$$\#1. n_b/n_0, \#2. n_b \text{ (fm}^{-3}\text{)}, \#3. Y_p, \#4. Y_n, \#5. Y_{e^-}, \#6. Y_{\mu^-}$$

- **Figure 2:**

**For Figure 2a:** The data files corresponding to the equation of state (EOS) of NS matter for different models shown in Figure 2a can be availed from the sub-folder ‘Fig2a’. The columns of the EOS files are given as;

$$\#1. n_b/n_0, \#2. n_b \text{ (fm}^{-3}\text{)}, \#3. \epsilon \text{ (MeV fm}^{-3}\text{)}, \#4. p \text{ (MeV fm}^{-3}\text{)}$$

$\epsilon$  is the energy density, and  $p$  is the pressure.

**For Figure 2b and 2c:** The data files for the mass ( $M$ )-radius ( $R$ ) configurations of NSs (Figure 2b) and the dimensionless tidal deformability parameter ( $\bar{\Lambda}$ ) for NSs corresponding to different EOS models shown in Figure 2a can be availed from the sub-folder ‘Fig2band2c’. The columns of the files are given as;

$$\#1. n_b/n_0, \#2. n_b \text{ (fm}^{-3}\text{)}, \#3. \epsilon_c \text{ (MeV fm}^{-3}\text{)}, \#4. p_c \text{ (MeV fm}^{-3}\text{)}, \#5. M(M_\odot), \#6. R \text{ (km)}, \#7. \bar{\Lambda}$$

Where  $\epsilon_c$  and  $p_c$  are the central energy density and central pressure, respectively.

- **Figure 3:**

**For Figure 3a:** The data files for the lower and upper bounds for the EOSs shown in Figure 3a are given in the sub-folder ‘Fig3a’, and the columns of the files are given as;

$$\#1. n_b/n_0, \#2. n_b \text{ (fm}^{-3}\text{)}, \#3. \epsilon \text{ (MeV fm}^{-3}\text{)}, \#4. p \text{ (MeV fm}^{-3}\text{)}$$

**For Figure 3b:** The data files for the upper and lower bounds in the mass ( $M$ )-radius ( $R$ ) configurations of NSs (Figure 3b) can be availed from the sub-folder ‘Fig3b’. The columns of the files are given as;

$$\#1. n_b/n_0, \#2. n_b \text{ (fm}^{-3}\text{)}, \#3. \epsilon_c \text{ (MeV fm}^{-3}\text{)}, \#4. p_c \text{ (MeV fm}^{-3}\text{)}, \#5. M(M_\odot), \#6. R \text{ (km)}, \#7. \bar{\Lambda}$$

- **Figure 4:** The correlation matrices shown at different fixed  $\zeta$  values are obtained using the posterior distribution of the nuclear parameters and NS properties in Figure 5. However, the resulting correlation matrices can be availed in the folder ‘Fig4’. A snapshot of the code has also been provided, demonstrating how to use the data files to obtain the correlation plots shown in the manuscript.
- **Figure 5:** We provide the data files for the displayed weighted posterior distribution of saturation parameters and NS properties corresponding to different constant  $\zeta$  EOS models in the folder ‘Fig5’. The columns of the files can be read as;

$$\#1. n_0 \text{ (fm}^{-3}\text{)}, \#2. E_{sat} \text{ (MeV)}, \#3. K \text{ (MeV)}, \#4. J \text{ (MeV)}, \#5. L \text{ (MeV)}, \#6. (\frac{m^*}{m_N}), \#7. \zeta, \\ \#8. M_{\max} (M_\odot), \#9. R_{1.4M_\odot} \text{ (km)}, \#10. \Lambda_{1.4M_\odot}, \#11. R_{2M_\odot} \text{ (km)}, \#12. \Lambda_{2M_\odot}, \#13. W$$

Where ‘ $W$ ’ is the non-normalized statistical weight factor resulting from the astrophysical measurements (see section 3.2 in the manuscript). A description of the other parameters can be found in the manuscript.

- **Figure 6:** The data for scatter points in Figure 6 are provided in the data file in folder ‘Fig6’. The columns of the files are given;

$$\#1. \zeta, \#2. M_{\max}(M_\odot), \#3. R_{1.4M_\odot} \text{ (km)}$$

- **Figure 7:** The correlation matrix displayed is obtained using the data given in Figure 8. However, the resulting data for the correlation matrix is provided in the folder ‘Fig7’. A snapshot of the code has also been provided, demonstrating how to use the data files to obtain the correlation plots shown in the manuscript.
- **Figure 8:** The data file for the displayed weighted posterior distribution of saturation parameters and NS properties under consideration of a uniform prior on  $\zeta$  is given in the folder ‘Fig8’. The columns of the file can be read as;

$$\#1. n_0 \text{ (fm}^{-3}\text{)}, \#2. E_{sat} \text{ (MeV)}, \#3. K \text{ (MeV)}, \#4. J \text{ (MeV)}, \#5. L \text{ (MeV)}, \#6. (\frac{m^*}{m_N}), \#7. \zeta, \\ \#8. M_{\max} (M_\odot), \#9. R_{1.4M_\odot} \text{ (km)}, \#10. \Lambda_{1.4M_\odot}, \#11. R_{2M_\odot} \text{ (km)}, \#12. \Lambda_{2M_\odot}, \#13. W$$

- **Figure 9:** The data files for the binding energy of the pure neutron matter (PNM) displayed in Figure 9a are given in the folder ‘Fig9a’. Files are named corresponding to the values of  $\zeta$ , e.g., for  $\zeta = 0.01$ , the data is given in the file named ‘PNM\_zeta\_0.01.out.’. The columns of the data files are given as;

$$\#1. n_b \text{ (fm}^{-3}\text{)}, \#2. \epsilon \text{ (MeV fm}^{-3}\text{)}, \#3. p \text{ (MeV fm}^{-3}\text{)}, \#4. E/A \text{ (MeV)}$$

The data for the correlation matrix shown in Fig 9b is given in the sub-folder ‘Fig9b’.
